# Supplementary material for: Analyzing laser-induced alignment of weakly-bound molecular aggregates
Source: arXiv:1808.01206 source file (2018-08-03)
Supplement: Supplementary file 1 [file indole_water_theory_supplemental.pdf]

# Supplemental Material: Analyzing laser-induced alignment of weakly-bound molecular aggregates

Linda V. Thesing,[1,2,3] Andrey Yachmenev,[1,2] Rosario González-Férez,[4,‖] and Jochen Küpper[1,2,3,*]

[1]*Center for Free-Electron Laser Science, Deutsches Elektronen-Synchrotron DESY, Notkestrasse 85, 22607 Hamburg, Germany*
[2]*The Hamburg Center for Ultrafast Imaging, Universität Hamburg, Luruper Chaussee 149, 22761 Hamburg, Germany*
[3]*Department of Physics, Universität Hamburg, Luruper Chaussee 149, 22761 Hamburg, Germany*
[4]*Instituto Carlos I de Física Teórica y Computacional and Departamento de Física Atómica, Molecular y Nuclear, Universidad de Granada, 18071 Granada, Spain*
(Dated: July 30, 2018)

## I. AB INITIO RESULTS

The *ab initio* results for the components of the EDM $\boldsymbol{\mu}(\tau)$ and polarizability $\underline{\underline{\alpha}}(\tau)$ are depicted in Fig. 1 together with the analytical functions fitted to the *ab initio* results, see section III. For each geometry obtained for a fixed value of the torsional angle, the EDM and polarizability are calculated as first and second derivatives of the electronic energy with respect to external electric fields along the corresponding axis. We use electric field strengths of +0.005 a. u.. and −0.005 a. u., where 1 a. u.. = $5.14 \times 10^9$ V/cm. As for the geometry optimization, the DF-MP2 method and aug-cc-pVTZ basis set is used.

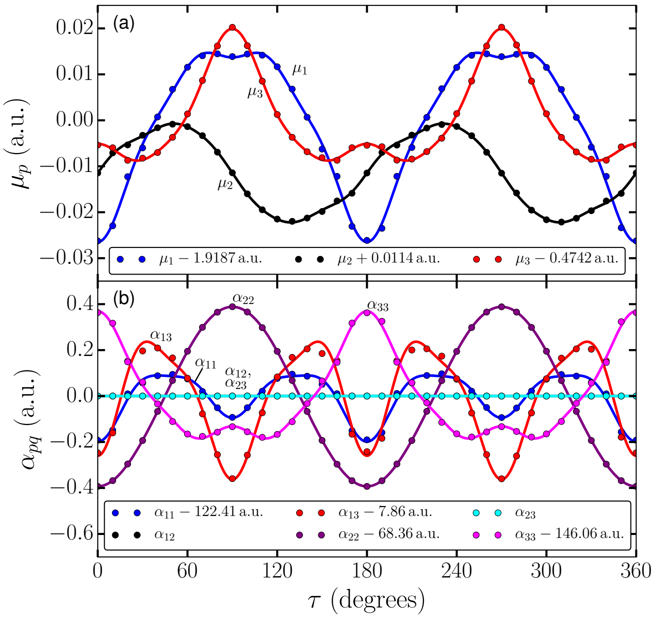


FIG. 1. The *ab initio* results for the components of (a) the EDM $\boldsymbol{\mu}(\tau)$ and (b) the polarizability $\underline{\underline{\alpha}}(\tau)$ (circles). The solid lines are the analytical functions fitted to the *ab initio* results, see section III.

## II. ANALYTICAL EXPRESSIONS FOR THE STRUCTURAL PARAMETERS

The bond lengths $r_i$, angles $a_i$, and dihedral angles $d_i$ of indole($H_2O$) are defined in Z-matrix form according to Table I, where $d_{18} = \tau$, $d_i = 0$ for $i \in \{4, 5, 7, 8, 9\}$ and $d_i = \pi$ for $i \in \{6, 10, 11, 12, 13, 14, 15, 16, 17, 19\}$. The coordinates $r_i$, $i \neq 18, 19$ and $a_i$, $i \neq 18$ are represented as analytical functions of the torsional angle similar to the potential energy surface

$$x_i = \sum_{n=0}^{3} x_{2n}^{(i)} \cos(2n\tau) \qquad (1)$$

to preserve their symmetry. To obtain expressions for $r_{18} = r_{\mathrm{OH}_1}$, $r_{19} = r_{\mathrm{OH}_2}$ and $a_{18} = a_{\mathrm{NOH}_1}$, we fit symmetrized coordinates defined as $r_+ = (r_{18} + r_{19})/2$, $r_- = (r_{18} - r_{19})/2$ and $a_- = a_{18} + 1/2a_{19} - \pi$, where $a_{19} = a_{\mathrm{HOH}}$. For $r_+$, the expression (1) is used and for $r_-$ and $a_-$ we fit

$$x_i = \sum_{n=0}^{2} x_{2n+1}^{(i)} \cos((2n+1)\tau) \; . \qquad (2)$$

Analytical expressions for the coordinates $r_{18}$, $r_{19}$ and $a_{18}$ are then obtained from those for the symmetrized coordinates. The coefficients $x_{2n}^{(i)}$ and $x_{2n+1}^{(i)}$ are listed in Table III.

## III. ANALYTICAL EXPRESSIONS FOR THE ELECTRIC DIPOLE MOMENT AND POLARIZABILITY

To represent $\boldsymbol{\mu}(\tau)$ and $\underline{\underline{\alpha}}(\tau)$ by analytical functions of $\tau$, we transform their components to a coordinate system fixed to the molecular bond structure. The first unit vector $\hat{e}_1$ is chosen along the N-O bond axis, the second one $\hat{e}_2$ is perpendicular to the indole plane and the third one is given by $\hat{e}_3 = \hat{e}_1 \times \hat{e}_2$. Similar to the fit of the PES, we fit the following expressions to the *ab initio* results of $\boldsymbol{\mu}(\tau)$ and $\underline{\underline{\alpha}}(\tau)$

$$\mu_p = \sum_{n=0}^{4} \mu_{2n}^{(p)} \cos(2n\tau) \; , \; \alpha_{pq} = \sum_{n=0}^{4} \alpha_{2n}^{(pq)} \cos(2n\tau) \qquad (3)$$

‖ rogonzal@ugr.es
* jochen.kuepper@cfel.de; https://www.controlled-molecule-imaging.org

| | | | | | | |
|---|---|---|---|---|---|---|
| C | | | | | | |
| C | 1 | $r_2$ | | | | |
| C | 2 | $r_3$ | 1 | $a_3$ | | |
| C | 3 | $r_4$ | 2 | $a_4$ | 1 | $d_4$ |
| N | 1 | $r_5$ | 2 | $a_5$ | 3 | $d_5$ |
| C | 2 | $r_6$ | 1 | $a_6$ | 3 | $d_6$ |
| C | 6 | $r_7$ | 2 | $a_7$ | 1 | $d_7$ |
| C | 7 | $r_8$ | 6 | $a_8$ | 2 | $d_8$ |
| C | 8 | $r_9$ | 7 | $a_9$ | 6 | $d_9$ |
| H | 3 | $r_{10}$ | 2 | $a_{10}$ | 1 | $d_{10}$ |
| H | 4 | $r_{11}$ | 3 | $a_{11}$ | 2 | $d_{11}$ |
| H | 6 | $r_{12}$ | 2 | $a_{12}$ | 1 | $d_{12}$ |
| H | 7 | $r_{13}$ | 6 | $a_{13}$ | 2 | $d_{13}$ |
| H | 8 | $r_{14}$ | 7 | $a_{14}$ | 6 | $d_{14}$ |
| H | 9 | $r_{15}$ | 8 | $a_{15}$ | 7 | $d_{15}$ |
| O | 5 | $r_{16}$ | 1 | $a_{16}$ | 2 | $d_{16}$ |
| H | 5 | $r_{17}$ | 1 | $a_{17}$ | 2 | $d_{17}$ |
| H | 16 | $r_{18}$ | 5 | $a_{18}$ | 1 | $d_{18}$ |
| H | 16 | $r_{19}$ | 18 | $a_{19}$ | 5 | $d_{19}$ |

TABLE I. Z-matrix for internal coordinates of indole($H_2O$) as used in the input of the ab initio calculations.

with $p \in \{1, 3\}$ and $pq \in \{11, 22, 33, 13\}$ as well as

$$\mu_2 = \sin(2\tau) \sum_{n=0}^{4} \mu_{2n}^{(p)} \cos(2n\tau) \ . \tag{4}$$

The coefficients $\mu_{2n}^{(p)}$ and $\alpha_{2n}^{(pq)}$ are listed in Table IV.

## IV. SYMMETRY PROPERTIES AND COUPLING DUE TO EXTERNAL ELECTRIC FIELDS

We summarize the symmetry properties of indole($H_2O$) and the coupling of different rotation-torsional states in the presence of parallel non-resonant laser and weak static electric fields. In the field-free case, indole($H_2O$) belongs to the molecular symmetry group $G_4 = \{E, (12), E^*, (12)^*\}$ [1–3]. The static electric field mixes field-free states of different parity and the molecular symmetry group of indole($H_2O$) in the field reduces to $G_2 = \{E, (12)\}$ [3]. In terms of the product states $\Psi_l^{rot}(\phi, \theta, \chi)\Psi_m^{tor}(\tau)$, the matrix elements of the two parts of the interaction Hamiltonian, (3) in the main text, depend on $\langle \Psi_m^{tor} | \mu_i(\tau) | \Psi_n^{tor} \rangle$ and $\langle \Psi_m^{tor} | \alpha_{ij}(\tau) | \Psi_n^{tor} \rangle$ with $i, j \in x, y, z$, respectively. Since the dipole moment and polarizability do not change sign under the operation (12), rotation-torsional states with different $\sigma$ are not coupled by the external ac and dc electric fields. The non-zero components of the polarizability are of $A_1$ symmetry in $G_4$ and thus only couple field-free torsional states that have the same symmetry. Since the field-free rotation-torsional states are linear combinations of states with the same rotation-torsional symmetry and only approximately described by product states, the coupling due to the laser field (which is the dominant interaction) between field-free states with different torsional symmetry are non-zero but smaller than the coupling between states with the same torsional symmetry. Here, the torsional symmetry of a field-free rotation-torsional state refers to the product state $\Psi_l^{rot}(\phi, \theta, \chi)\Psi_m^{tor}(\tau)$ with the largest contribution. For parallel laser and static electric fields, $M$ is a good quantum number and we have to distinguish the cases $M = 0$ and $M \neq 0$.

| $J$ | $K_c$ | $\Gamma_{\text{tor}}$ | $\Gamma_{\text{rot}} \otimes \Gamma_{\text{tor}}$ | symmetry species |
|---|---|---|---|---|
| $e$ | $e$ | $A_1$ | $A_1$ | + |
| $o$ | $e$ | $A_1$ | $A_1$ | − |
| $e$ | $o$ | $A_1$ | $A_2$ | − |
| $o$ | $o$ | $A_1$ | $A_2$ | + |
| $e$ | $e$ | $A_2$ | $A_2$ | − |
| $o$ | $e$ | $A_2$ | $A_2$ | + |
| $e$ | $o$ | $A_2$ | $A_1$ | + |
| $o$ | $o$ | $A_2$ | $A_1$ | − |

TABLE II. Symmetry species + and − for $M = 0$ and $\sigma = 0$ in the presence of parallel ac and dc electric fields. The torsional symmetry $\Gamma_{\text{tor}}$ and $K_c$ quantum number refer to the product state $\Psi_l^{rot}(\phi, \theta, \chi)\Psi_m^{tor}(\tau)$ that approximately describes a given field-free rotation-torsional state. To obtain the $M = 0$ symmetry species for the $\sigma = 1$ sublevels, $A_{1,2}$ has to be replaced with $B_{1,2}$.

If $M \neq 0$, we find two different symmetry species corresponding to states with A and B symmetry in $G_2$.

For $M = 0$, the interaction of the laser field with the polarizability as well as the interaction of the static electric field with the $y$- and $z$-components of the dipole moment couple field-free rotational states with the same $J + K_c$ parity. The $y$- and $z$-components of the dipole moment are of $A_1$ symmetry in $G_4$ and thus only couple field-free torsional states with the same symmetry. The $x$-component of the dipole moment is of $A_2$ symmetry and couples field-free torsional states with different parity, i. e., $A_1$ and $A_2$ torsional states as well as $B_1$ and $B_2$ states. For $M = 0$, the interaction with the $x$-component of the dipole moment couples field-free rotational states with different $J + K_c$ parity. As a consequence, we find two different symmetry species for each value of $\sigma$. The two cases for $\sigma = 0$ are listed in Table II.

| $x_i$ | $x_0^{(i)}$ | $x_1^{(i)}$ | $x_2^{(i)}$ | $x_3^{(i)}$ | $x_4^{(i)}$ | $x_5^{(i)}$ | $x_6^{(i)}$ |
|---|---|---|---|---|---|---|---|
| $r_2$ | 1.4165 | 0.0000 | $1.1241 \cdot 10^{-4}$ | 0.0000 | $-2.4354 \cdot 10^{-5}$ | 0.0000 | $7.9153 \cdot 10^{-7}$ |
| $r_3$ | 1.4190 | 0.0000 | $-1.5673 \cdot 10^{-4}$ | 0.0000 | $-6.2654 \cdot 10^{-6}$ | 0.0000 | $-2.3140 \cdot 10^{-6}$ |
| $r_4$ | 1.3723 | 0.0000 | $-5.2534 \cdot 10^{-6}$ | 0.0000 | $1.1913 \cdot 10^{-5}$ | 0.0000 | $-2.0983 \cdot 10^{-6}$ |
| $r_5$ | 1.3653 | 0.0000 | $-1.9057 \cdot 10^{-4}$ | 0.0000 | $-1.8848 \cdot 10^{-5}$ | 0.0000 | $-4.9656 \cdot 10^{-6}$ |
| $r_6$ | 1.3996 | 0.0000 | $-1.9349 \cdot 10^{-5}$ | 0.0000 | $1.2147 \cdot 10^{-6}$ | 0.0000 | $-2.3413 \cdot 10^{-6}$ |
| $r_7$ | 1.3798 | 0.0000 | $-3.3917 \cdot 10^{-5}$ | 0.0000 | $3.2087 \cdot 10^{-6}$ | 0.0000 | $-7.9436 \cdot 10^{-7}$ |
| $r_8$ | 1.4048 | 0.0000 | $-5.2823 \cdot 10^{-5}$ | 0.0000 | $-1.4796 \cdot 10^{-6}$ | 0.0000 | $-4.7037 \cdot 10^{-6}$ |
| $r_9$ | 1.3811 | 0.0000 | $-4.8092 \cdot 10^{-5}$ | 0.0000 | $1.2176 \cdot 10^{-5}$ | 0.0000 | $3.4123 \cdot 10^{-6}$ |
| $r_{10}$ | 1.0751 | 0.0000 | $-1.4861 \cdot 10^{-5}$ | 0.0000 | $-1.0067 \cdot 10^{-6}$ | 0.0000 | $-4.9208 \cdot 10^{-7}$ |
| $r_{11}$ | 1.0752 | 0.0000 | $-5.7300 \cdot 10^{-6}$ | 0.0000 | $-4.9008 \cdot 10^{-6}$ | 0.0000 | $-2.9040 \cdot 10^{-6}$ |
| $r_{12}$ | 1.0798 | 0.0000 | $-2.7355 \cdot 10^{-6}$ | 0.0000 | $3.3204 \cdot 10^{-6}$ | 0.0000 | $2.1854 \cdot 10^{-6}$ |
| $r_{13}$ | 1.0797 | 0.0000 | $-1.7141 \cdot 10^{-5}$ | 0.0000 | $8.4508 \cdot 10^{-6}$ | 0.0000 | $1.3853 \cdot 10^{-6}$ |
| $r_{14}$ | 1.0795 | 0.0000 | $6.4960 \cdot 10^{-7}$ | 0.0000 | $-2.0485 \cdot 10^{-5}$ | 0.0000 | $-1.7834 \cdot 10^{-6}$ |
| $r_{15}$ | 1.0800 | 0.0000 | $1.9670 \cdot 10^{-5}$ | 0.0000 | $8.2218 \cdot 10^{-6}$ | 0.0000 | $6.9811 \cdot 10^{-7}$ |
| $r_{16}$ | 2.9378 | 0.0000 | $1.4169 \cdot 10^{-2}$ | 0.0000 | $-1.2038 \cdot 10^{-4}$ | 0.0000 | $-4.9276 \cdot 10^{-5}$ |
| $r_{17}$ | 1.0090 | 0.0000 | $4.6907 \cdot 10^{-5}$ | 0.0000 | $4.8672 \cdot 10^{-7}$ | 0.0000 | $3.1249 \cdot 10^{-6}$ |
| $r_{18}$ | $9.5964 \cdot 10^{-1}$ | $1.6137 \cdot 10^{-5}$ | $-3.7570 \cdot 10^{-5}$ | $-2.3695 \cdot 10^{-6}$ | $-1.7981 \cdot 10^{-5}$ | $7.0582 \cdot 10^{-7}$ | $-2.5055 \cdot 10^{-6}$ |
| $r_{19}$ | $9.5964 \cdot 10^{-1}$ | $-1.6137 \cdot 10^{-5}$ | $-3.7570 \cdot 10^{-5}$ | $2.3695 \cdot 10^{-6}$ | $-1.7981 \cdot 10^{-5}$ | $-7.0582 \cdot 10^{-7}$ | $-2.5055 \cdot 10^{-6}$ |
| $a_3$ | 1.8649 | 0.0000 | $3.7557 \cdot 10^{-5}$ | 0.0000 | $-5.1228 \cdot 10^{-5}$ | 0.0000 | $-1.1234 \cdot 10^{-6}$ |
| $a_4$ | 1.8647 | 0.0000 | $-1.7675 \cdot 10^{-4}$ | 0.0000 | $4.1198 \cdot 10^{-5}$ | 0.0000 | $1.2049 \cdot 10^{-6}$ |
| $a_5$ | 1.8773 | 0.0000 | $1.8366 \cdot 10^{-6}$ | 0.0000 | $6.5937 \cdot 10^{-5}$ | 0.0000 | $1.5983 \cdot 10^{-6}$ |
| $a_6$ | 2.0751 | 0.0000 | $2.8057 \cdot 10^{-4}$ | 0.0000 | $-3.9346 \cdot 10^{-5}$ | 0.0000 | $1.3686 \cdot 10^{-5}$ |
| $a_7$ | 2.0749 | 0.0000 | $2.0874 \cdot 10^{-4}$ | 0.0000 | $2.1963 \cdot 10^{-6}$ | 0.0000 | $2.3899 \cdot 10^{-6}$ |
| $a_8$ | 2.1167 | 0.0000 | $-1.8787 \cdot 10^{-4}$ | 0.0000 | $2.3553 \cdot 10^{-5}$ | 0.0000 | $-3.4979 \cdot 10^{-6}$ |
| $a_9$ | 2.1152 | 0.0000 | $-2.1611 \cdot 10^{-4}$ | 0.0000 | $-2.4107 \cdot 10^{-5}$ | 0.0000 | $-6.0503 \cdot 10^{-6}$ |
| $a_{10}$ | 2.2269 | 0.0000 | $-1.1047 \cdot 10^{-4}$ | 0.0000 | $4.6785 \cdot 10^{-5}$ | 0.0000 | $-1.6861 \cdot 10^{-5}$ |
| $a_{11}$ | 2.2678 | 0.0000 | $-7.3596 \cdot 10^{-4}$ | 0.0000 | $-3.7692 \cdot 10^{-5}$ | 0.0000 | $1.2068 \cdot 10^{-5}$ |
| $a_{12}$ | 2.1047 | 0.0000 | $-1.6749 \cdot 10^{-4}$ | 0.0000 | $2.1358 \cdot 10^{-5}$ | 0.0000 | $1.1809 \cdot 10^{-6}$ |
| $a_{13}$ | 2.0896 | 0.0000 | $1.6504 \cdot 10^{-4}$ | 0.0000 | $-7.4212 \cdot 10^{-6}$ | 0.0000 | $-2.8143 \cdot 10^{-7}$ |
| $a_{14}$ | 2.0825 | 0.0000 | $1.8096 \cdot 10^{-4}$ | 0.0000 | $6.1563 \cdot 10^{-5}$ | 0.0000 | $8.5536 \cdot 10^{-6}$ |
| $a_{15}$ | 2.1148 | 0.0000 | $-1.8007 \cdot 10^{-3}$ | 0.0000 | $2.2403 \cdot 10^{-4}$ | 0.0000 | $-4.2819 \cdot 10^{-5}$ |
| $a_{16}$ | 2.1705 | 0.0000 | $-2.6675 \cdot 10^{-4}$ | 0.0000 | $-8.9622 \cdot 10^{-3}$ | 0.0000 | $-1.2984 \cdot 10^{-3}$ |
| $a_{17}$ | 2.1885 | 0.0000 | $8.9775 \cdot 10^{-4}$ | 0.0000 | $-9.4758 \cdot 10^{-4}$ | 0.0000 | $1.1903 \cdot 10^{-5}$ |
| $a_{18}$ | 2.2242 | $-4.7488 \cdot 10^{-2}$ | $9.8120 \cdot 10^{-4}$ | $-1.5970 \cdot 10^{-3}$ | $-4.1175 \cdot 10^{-5}$ | $-4.0832 \cdot 10^{-3}$ | $1.0285 \cdot 10^{-5}$ |
| $a_{19}$ | 1.8347 | 0.0000 | $-1.9624 \cdot 10^{-3}$ | 0.0000 | $8.2349 \cdot 10^{-5}$ | 0.0000 | $-2.0570 \cdot 10^{-5}$ |

TABLE III. Coefficients of the analytical functions (1) and (2) used to fit the internal coordinates computed with *ab initio* methods.

| $n$ | $\mu_{2n}^{(1)}$ (a.u.) | $\mu_{2n}^{(2)}$ (a.u.) | $\mu_{2n}^{(3)}$ (a.u.) | $\alpha_{2n}^{(11)}$ (a.u.) | $\alpha_{2n}^{(13)}$ (a.u.) | $\alpha_{2n}^{(22)}$ (a.u.) | $\alpha_{2n}^{(33)}$ (a.u.) |
|---|---|---|---|---|---|---|---|
| 0 | 1.91872 | $1.146652 \cdot 10^{-2}$ | $4.742808 \cdot 10^{-1}$ | 122.4133 | 7.866651 | 68.36602 | 146.069 |
| 1 | $1.897090 \cdot 10^{-2}$ | $1.110871 \cdot 10^{-3}$ | $1.161703 \cdot 10^{-2}$ | $3.613539 \cdot 10^{-2}$ | $8.455194 \cdot 10^{-2}$ | $3.895537 \cdot 10^{-1}$ | $2.378808 \cdot 10^{-1}$ |
| 2 | $4.952774 \cdot 10^{-3}$ | $1.531671 \cdot 10^{-3}$ | $6.384580 \cdot 10^{-3}$ | $1.17512 \cdot 10^{-1}$ | $2.451433 \cdot 10^{-1}$ | $-1.195350 \cdot 10^{-3}$ | $9.374843 \cdot 10^{-2}$ |
| 3 | $1.113748 \cdot 10^{-3}$ | $6.033855 \cdot 10^{-4}$ | $8.993579 \cdot 10^{-4}$ | $1.584098 \cdot 10^{-2}$ | $3.293678 \cdot 10^{-2}$ | $1.155859 \cdot 10^{-3}$ | $1.251454 \cdot 10^{-2}$ |
| 4 | $1.443935 \cdot 10^{-3}$ | $5.059124 \cdot 10^{-4}$ | $1.0173 \cdot 10^{-3}$ | $2.897917 \cdot 10^{-2}$ | $6.613491 \cdot 10^{-2}$ | $-1.084440 \cdot 10^{-3}$ | $2.512222 \cdot 10^{-2}$ |

TABLE IV. Coefficients of the analytical functions (3) and (4) used to fit the EDM and polarizability computed with *ab initio* methods. The components $\alpha_{12}$ and $\alpha_{23}$ are zero.

| $n$ | $\tilde{\alpha}_n^{(11)}$ (a. u.) | $\tilde{\alpha}_n^{(13)}$ (a. u.) | $\tilde{\alpha}_n^{(22)}$ (a. u.) | $\tilde{\alpha}_n^{(33)}$ (a. u.) |
|---|---|---|---|---|
| 0 | 98.8163 | 56.5324 | -9.156292 | 193.5136 |
| 1 | -23.5024 | 4.902866 | -77.91074 | 47.57616 |

TABLE V. Coefficients of the analytical functions (3) used to fit the modified polarizability. The components $\alpha_{12}$ and $\alpha_{23}$ are zero.


[1] G. Berden, W. L. Meerts, M. Schmitt, and K. Kleinermanns, "High resolution UV spectroscopy of phenol and the hydrogen bonded phenol-water cluster," J. Chem. Phys. **104**, 972 (1996).

[2] T. M. Korter, D. W. Pratt, and J. Küpper, "Indole-$H_2O$ in the gas phase. Structures, barriers to internal motion, and $S_1 \leftarrow S_0$ transition moment orientation. Solvent reorganization in the electronically excited state," J. Phys. Chem. A **102**, 7211–7216 (1998).

[3] S. Trippel, Y.-P. Chang, S. Stern, T. Mullins, L. Holmegaard, and J. Küpper, "Spatial separation of state- and size-selected neutral clusters," Phys. Rev. A **86**, 033202 (2012), arXiv:1208.4935 [physics].
